# Supplementary material for: Assessing Code Generation with Intermediate Languages
Source: arXiv:2407.05411 source file (2024-07-07)
Supplement: Supplementary file 1 [file appendix-old.tex]

\clearpage
\newpage
\section{Appendix}
We present the additional experiment results. Table~\ref{tab:GTresults} shows the experiment results for intermediate-ground-truth to target generation for different models. Table~\ref{tab:corr1} to Table~\ref{tab:corrphi} present more correlation statistics. 
\begin{table}[!htp]\centering
\caption{Intermediate-ground-truth to Target generation}\label{tab:GTresults}
\scriptsize
\begin{tabular}{lrrrrrr}\toprule
\cellcolor[HTML]{d9ead3}GPT35 &\cellcolor[HTML]{d9ead3}cpp &\cellcolor[HTML]{d9ead3}go &\cellcolor[HTML]{d9ead3}java &\cellcolor[HTML]{d9ead3}python &\cellcolor[HTML]{d9ead3}rust \\\midrule
\cellcolor[HTML]{d9ead3}cpp & &74.39\% &71.95\% &85.98\% &71.34\% \\
\cellcolor[HTML]{d9ead3}go &69.51\% & &71.34\% &89.63\% &71.95\% \\
\cellcolor[HTML]{d9ead3}java &74.39\% &72.56\% & &85.98\% &65.85\% \\
\cellcolor[HTML]{d9ead3}python &68.29\% &72.56\% &67.68\% & &68.29\% \\
\cellcolor[HTML]{d9ead3}rust &73.17\% &65.85\% &73.78\% &85.37\% & \\
& & & & & \\
\cellcolor[HTML]{d9ead3}CodeLlama-7b &\cellcolor[HTML]{d9ead3}cpp &\cellcolor[HTML]{d9ead3}go &\cellcolor[HTML]{d9ead3}java &\cellcolor[HTML]{d9ead3}python &\cellcolor[HTML]{d9ead3}rust \\
\cellcolor[HTML]{d9ead3}cpp & &44.51\% &57.93\% &54.27\% &25.00\% \\
\cellcolor[HTML]{d9ead3}go &47.56\% & &54.88\% &62.80\% &27.44\% \\
\cellcolor[HTML]{d9ead3}java &48.17\% &43.90\% & &62.20\% &25.00\% \\
\cellcolor[HTML]{d9ead3}python &44.51\% &39.02\% &47.56\% & &25.00\% \\
\cellcolor[HTML]{d9ead3}rust &39.63\% &35.37\% &42.68\% &51.83\% & \\
& & & & & \\
\cellcolor[HTML]{d9ead3}CodeLlama-13b &\cellcolor[HTML]{d9ead3}cpp &\cellcolor[HTML]{d9ead3}go &\cellcolor[HTML]{d9ead3}java &\cellcolor[HTML]{d9ead3}python &\cellcolor[HTML]{d9ead3}rust \\
\cellcolor[HTML]{d9ead3}cpp & &42.68\% &57.93\% &47.56\% &30.49\% \\
\cellcolor[HTML]{d9ead3}go &48.78\% & &57.32\% &58.54\% &32.32\% \\
\cellcolor[HTML]{d9ead3}java &47.56\% &46.34\% & &62.20\% &34.76\% \\
\cellcolor[HTML]{d9ead3}python &45.12\% &41.46\% &51.22\% & &23.78\% \\
\cellcolor[HTML]{d9ead3}rust &48.17\% &36.59\% &53.05\% &45.73\% & \\
& & & & & \\
\cellcolor[HTML]{d9ead3}CodeLlama-34b &\cellcolor[HTML]{d9ead3}cpp &\cellcolor[HTML]{d9ead3}go &\cellcolor[HTML]{d9ead3}java &\cellcolor[HTML]{d9ead3}python &\cellcolor[HTML]{d9ead3}rust \\
\cellcolor[HTML]{d9ead3}cpp & &39.02\% &53.05\% &58.54\% &31.10\% \\
\cellcolor[HTML]{d9ead3}go &79.27\% & &58.54\% &62.20\% &31.10\% \\
\cellcolor[HTML]{d9ead3}java &52.44\% &44.51\% & &60.98\% &34.15\% \\
\cellcolor[HTML]{d9ead3}python &48.78\% &42.07\% &53.05\% & &32.93\% \\
\cellcolor[HTML]{d9ead3}rust &46.95\% &43.90\% &52.44\% &53.05\% & \\
& & & & & \\
\cellcolor[HTML]{d9ead3}CodeLlama-70b &\cellcolor[HTML]{d9ead3}cpp &\cellcolor[HTML]{d9ead3}go &\cellcolor[HTML]{d9ead3}java &\cellcolor[HTML]{d9ead3}python &\cellcolor[HTML]{d9ead3}rust \\
\cellcolor[HTML]{d9ead3}cpp & &54.88\% &67.07\% &67.68\% &32.32\% \\
\cellcolor[HTML]{d9ead3}go &54.88\% & &70.12\% &68.90\% &29.88\% \\
\cellcolor[HTML]{d9ead3}java &54.88\% &56.71\% & &67.07\% &30.49\% \\
\cellcolor[HTML]{d9ead3}python &56.10\% &53.66\% &72.56\% & &31.10\% \\
\cellcolor[HTML]{d9ead3}rust &56.10\% &51.22\% &68.90\% &65.85\% & \\
& & & & & \\
\cellcolor[HTML]{d9ead3}Mixtral 8x7b &\cellcolor[HTML]{d9ead3}cpp &\cellcolor[HTML]{d9ead3}go &\cellcolor[HTML]{d9ead3}java &\cellcolor[HTML]{d9ead3}python &\cellcolor[HTML]{d9ead3}rust \\
\cellcolor[HTML]{d9ead3}cpp & &57.93\% &73.17\% &66.46\% &48.78\% \\
\cellcolor[HTML]{d9ead3}go &60.98\% & &76.83\% &51.83\% &43.29\% \\
\cellcolor[HTML]{d9ead3}java &60.37\% &62.20\% & &78.66\% &56.71\% \\
\cellcolor[HTML]{d9ead3}python &56.10\% &60.37\% &71.34\% & &42.07\% \\
\cellcolor[HTML]{d9ead3}rust &59.15\% &62.80\% &70.12\% &70.12\% & \\
& & & & & \\
\cellcolor[HTML]{d9ead3}Deepseek &\cellcolor[HTML]{d9ead3}cpp &\cellcolor[HTML]{d9ead3}go &\cellcolor[HTML]{d9ead3}java &\cellcolor[HTML]{d9ead3}python &\cellcolor[HTML]{d9ead3}rust \\
\cellcolor[HTML]{d9ead3}cpp & &44.51\% &65.24\% &65.24\% &28.05\% \\
\cellcolor[HTML]{d9ead3}go &51.22\% & &65.85\% &70.73\% &28.66\% \\
\cellcolor[HTML]{d9ead3}java &59.76\% &48.17\% & &73.78\% &29.88\% \\
\cellcolor[HTML]{d9ead3}python &51.83\% &43.29\% &66.46\% & &25.61\% \\
\cellcolor[HTML]{d9ead3}rust &57.32\% &39.02\% &62.80\% &60.37\% & \\
& & & & & \\
\cellcolor[HTML]{d9ead3}Stable &\cellcolor[HTML]{d9ead3}cpp &\cellcolor[HTML]{d9ead3}go &\cellcolor[HTML]{d9ead3}java &\cellcolor[HTML]{d9ead3}python &\cellcolor[HTML]{d9ead3}rust \\
\cellcolor[HTML]{d9ead3}cpp & &38.41\% &49.39\% &55.49\% &22.56\% \\
\cellcolor[HTML]{d9ead3}go &36.59\% & &48.17\% &35.98\% &20.12\% \\
\cellcolor[HTML]{d9ead3}java &39.02\% &41.46\% & &57.32\% &24.39\% \\
\cellcolor[HTML]{d9ead3}python &34.76\% &38.41\% &54.88\% & &23.17\% \\
\cellcolor[HTML]{d9ead3}rust &37.80\% &35.98\% &45.73\% &57.93\% & \\
& & & & & \\
\cellcolor[HTML]{d9ead3}Phi &\cellcolor[HTML]{d9ead3}cpp &\cellcolor[HTML]{d9ead3}go &\cellcolor[HTML]{d9ead3}java &\cellcolor[HTML]{d9ead3}python &\cellcolor[HTML]{d9ead3}rust \\
\cellcolor[HTML]{d9ead3}cpp & &32.93\% &54.27\% &62.20\% &11.59\% \\
\cellcolor[HTML]{d9ead3}go &39.02\% & &25.00\% &65.24\% &13.41\% \\
\cellcolor[HTML]{d9ead3}java &37.80\% &19.51\% & &50.61\% &15.85\% \\
\cellcolor[HTML]{d9ead3}python &43.29\% &29.27\% &40.24\% & &11.59\% \\
\cellcolor[HTML]{d9ead3}rust &39.02\% &26.22\% &43.29\% &65.85\% & \\
\bottomrule
\end{tabular}
\end{table}

\begin{table}[!htp]\centering
\caption{Correlation of model's translation ability and intermediate-target prompting}\label{tab:corr1}
\scriptsize
    \centering
    \begin{tabular}{c|c|c|c|c|c|c|c|c}\toprule
         GPT35 & CodeLlama7b & CodeLlama13b & CodeLlama34b& CodeLlama70b& Mixtral8x7b& Deepseek1.3b & Stable3b &Phi3.8b \\\midrule
         72.2\% & 89.7\% & 75.0\% & 90.9\%& 97.7\% & 84.9\%& 86.7\% & 81.6\% & 88.9\%
    \end{tabular}
\end{table}

\begin{table}[!htp]\centering
\caption{Correlation of model's translation ability and intermediate-target prompting}\label{tab:corr1}
\scriptsize
    \centering
    \begin{tabular}{c|c|c|c|c|c|c|c|c}\toprule
         GPT35 & CodeLlama7b & CodeLlama13b & CodeLlama34b& CodeLlama70b& Mixtral8x7b& Deepseek1.3b & Stable3b &Phi3.8b \\\midrule
         72.2\% & 89.7\% & 75.0\% & 90.9\%& 97.7\% & 84.9\%& 86.7\% & 81.6\% & 88.9\%
    \end{tabular}
\end{table}

\begin{table}[!htp]\centering
\caption{GPT3}\label{tab:corrgpt3}
\scriptsize
\begin{tabular}{lrrrrr}\toprule
\textbf{X-CPP vs Cpp-X} &\textbf{X-Go vs Go-X} &\textbf{X-Java vs Java-X} &\textbf{X-Python vs Python-X} &\textbf{X-Rust vs Rust-X} \\
97.6\% &93.3\% &-62.0\% &67.6\% &-83.7\% \\
\textbf{X vs X-CPP} &\textbf{X vs X-Go} &\textbf{X vs X-Java} &\textbf{X vs X-Python} &\textbf{X vs X-Rust} \\
89.8\% &87.0\% &-64.9\% &68.8\% &-75.6\% \\
\textbf{X vs CPP-X} &\textbf{X vs Go-X} &\textbf{X vs Java-X} &\textbf{X vs Python-X} &\textbf{X vs Rust-X} \\
78.7\% &80.5\% &99.8\% &99.9\% &53.0\% \\
\bottomrule
\end{tabular}
\end{table}


\begin{table}[!htp]\centering
\caption{GPT4}\label{tab:corrgpt4}
\scriptsize
\begin{tabular}{lrrrrr}\toprule
\textbf{X-CPP vs Cpp-X} &\textbf{X-Go vs Go-X} &\textbf{X-Java vs Java-X} &\textbf{X-Python vs Python-X} &\textbf{X-Rust vs Rust-X} \\
38.5\% &-60.0\% &-47.1\% &55.1\% &56.3\% \\
\textbf{X vs X-CPP} &\textbf{X vs X-Go} &\textbf{X vs X-Java} &\textbf{X vs X-Python} &\textbf{X vs X-Rust} \\
20.9\% &-54.9\% &-18.6\% &11.5\% &21.5\% \\
\textbf{X vs CPP-X} &\textbf{X vs Go-X} &\textbf{X vs Java-X} &\textbf{X vs Python-X} &\textbf{X vs Rust-X} \\
96.2\% &98.1\% &93.7\% &84.5\% &92.7\% \\
\bottomrule
\end{tabular}
\end{table}


\begin{table}[!htp]\centering
\caption{CodeLlama7b}\label{tab:corr7b}
\scriptsize
\begin{tabular}{lrrrrr}\toprule
\textbf{X-CPP vs Cpp-X} &\textbf{X-Go vs Go-X} &\textbf{X-Java vs Java-X} &\textbf{X-Python vs Python-X} &\textbf{X-Rust vs Rust-X} \\
-28.0\% &-51.7\% &-46.6\% &40.0\% &-22.1\% \\
\textbf{X vs X-CPP} &\textbf{X vs X-Go} &\textbf{X vs X-Java} &\textbf{X vs X-Python} &\textbf{X vs X-Rust} \\
23.7\% &-47.2\% &-59.2\% &45.2\% &-21.9\% \\
\textbf{X vs CPP-X} &\textbf{X vs Go-X} &\textbf{X vs Java-X} &\textbf{X vs Python-X} &\textbf{X vs Rust-X} \\
85.4\% &97.4\% &98.2\% &99.8\% &97.6\% \\
\bottomrule
\end{tabular}
\end{table}


\begin{table}[!htp]\centering
\caption{CodeLlama13b}\label{tab:corr13b}
\scriptsize
\begin{tabular}{lrrrrr}\toprule
\textbf{X-CPP vs Cpp-X} &\textbf{X-Go vs Go-X} &\textbf{X-Java vs Java-X} &\textbf{X-Python vs Python-X} &\textbf{X-Rust vs Rust-X} \\
-35.5\% &-80.8\% &-3.3\% &-98.3\% &12.9\% \\
\textbf{X vs X-CPP} &\textbf{X vs X-Go} &\textbf{X vs X-Java} &\textbf{X vs X-Python} &\textbf{X vs X-Rust} \\
-54.7\% &-83.2\% &-15.5\% &-96.0\% &32.2\% \\
\textbf{X vs CPP-X} &\textbf{X vs Go-X} &\textbf{X vs Java-X} &\textbf{X vs Python-X} &\textbf{X vs Rust-X} \\
97.7\% &99.9\% &98.2\% &99.1\% &98.0\% \\
\bottomrule
\end{tabular}
\end{table}


\begin{table}[!htp]\centering
\caption{CodeLlama34b}\label{tab:corr34b}
\scriptsize
\begin{tabular}{lrrrrr}\toprule
\textbf{X-CPP vs Cpp-X} &\textbf{X-Go vs Go-X} &\textbf{X-Java vs Java-X} &\textbf{X-Python vs Python-X} &\textbf{X-Rust vs Rust-X} \\
-91.8\% &-13.3\% &27.0\% &-26.9\% &-66.1\% \\
\textbf{X vs X-CPP} &\textbf{X vs X-Go} &\textbf{X vs X-Java} &\textbf{X vs X-Python} &\textbf{X vs X-Rust} \\
-93.9\% &-32.1\% &4.1\% &-64.0\% &-72.5\% \\
\textbf{X vs CPP-X} &\textbf{X vs Go-X} &\textbf{X vs Java-X} &\textbf{X vs Python-X} &\textbf{X vs Rust-X} \\
94.6\% &98.0\% &97.3\% &91.2\% &96.8\% \\
\bottomrule
\end{tabular}
\end{table}


\begin{table}[!htp]\centering
\caption{CodeLlama70b}\label{tab:corr70b}
\scriptsize
\begin{tabular}{lrrrrr}\toprule
\textbf{X-CPP vs Cpp-X} &\textbf{X-Go vs Go-X} &\textbf{X-Java vs Java-X} &\textbf{X-Python vs Python-X} &\textbf{X-Rust vs Rust-X} \\
-28.9\% &-86.6\% &-99.3\% &34.5\% &-59.8\% \\
\textbf{X vs X-CPP} &\textbf{X vs X-Go} &\textbf{X vs X-Java} &\textbf{X vs X-Python} &\textbf{X vs X-Rust} \\
-16.4\% &-83.5\% &-95.3\% &9.1\% &-69.5\% \\
\textbf{X vs CPP-X} &\textbf{X vs Go-X} &\textbf{X vs Java-X} &\textbf{X vs Python-X} &\textbf{X vs Rust-X} \\
99.2\% &99.7\% &97.1\% &96.5\% &97.3\% \\
\bottomrule
\end{tabular}
\end{table}


\begin{table}[!htp]\centering
\caption{Mixtral7b}\label{tab:corrm7}
\scriptsize
\begin{tabular}{lrrrrr}\toprule
\textbf{X-CPP vs Cpp-X} &\textbf{X-Go vs Go-X} &\textbf{X-Java vs Java-X} &\textbf{X-Python vs Python-X} &\textbf{X-Rust vs Rust-X} \\
38.5\% &64.0\% &-7.7\% &99.9\% &94.9\% \\
\textbf{X vs X-CPP} &\textbf{X vs X-Go} &\textbf{X vs X-Java} &\textbf{X vs X-Python} &\textbf{X vs X-Rust} \\
28.5\% &68.0\% &-16.6\% &98.0\% &90.5\% \\
\textbf{X vs CPP-X} &\textbf{X vs Go-X} &\textbf{X vs Java-X} &\textbf{X vs Python-X} &\textbf{X vs Rust-X} \\
94.6\% &99.8\% &99.4\% &98.5\% &98.3\% \\
\bottomrule
\end{tabular}
\end{table}


\begin{table}[!htp]\centering
\caption{Mixtral8x7b}\label{tab:corrm8}
\scriptsize
\begin{tabular}{lrrrrr}\toprule
\textbf{X-CPP vs Cpp-X} &\textbf{X-Go vs Go-X} &\textbf{X-Java vs Java-X} &\textbf{X-Python vs Python-X} &\textbf{X-Rust vs Rust-X} \\
28.5\% &88.7\% &43.6\% &-56.0\% &-39.1\% \\
\textbf{X vs X-CPP} &\textbf{X vs X-Go} &\textbf{X vs X-Java} &\textbf{X vs X-Python} &\textbf{X vs X-Rust} \\
62.0\% &78.2\% &23.1\% &0.5\% &-22.0\% \\
\textbf{X vs CPP-X} &\textbf{X vs Go-X} &\textbf{X vs Java-X} &\textbf{X vs Python-X} &\textbf{X vs Rust-X} \\
91.7\% &91.1\% &89.4\% &82.5\% &63.4\% \\
\bottomrule
\end{tabular}
\end{table}


\begin{table}[!htp]\centering
\caption{Deepseek-1.3b}\label{tab:corrdeep}
\scriptsize
\begin{tabular}{lrrrrr}\toprule
\textbf{X-CPP vs Cpp-X} &\textbf{X-Go vs Go-X} &\textbf{X-Java vs Java-X} &\textbf{X-Python vs Python-X} &\textbf{X-Rust vs Rust-X} \\
-48.8\% &-14.3\% &63.6\% &-75.0\% &86.7\% \\
\textbf{X vs X-CPP} &\textbf{X vs X-Go} &\textbf{X vs X-Java} &\textbf{X vs X-Python} &\textbf{X vs X-Rust} \\
-50.5\% &1.2\% &93.9\% &-51.8\% &80.1\% \\
\textbf{X vs CPP-X} &\textbf{X vs Go-X} &\textbf{X vs Java-X} &\textbf{X vs Python-X} &\textbf{X vs Rust-X} \\
99.6\% &93.5\% &86.3\% &93.9\% &99.2\% \\
\bottomrule
\end{tabular}
\end{table}



\begin{table}[!htp]\centering
\caption{Stable3b}\label{tab:corrstable}
\scriptsize
\begin{tabular}{lrrrrr}\toprule
\textbf{X-CPP vs Cpp-X} &\textbf{X-Go vs Go-X} &\textbf{X-Java vs Java-X} &\textbf{X-Python vs Python-X} &\textbf{X-Rust vs Rust-X} \\
-31.5\% &10.0\% &-34.2\% &-84.1\% &48.8\% \\
\textbf{X vs X-CPP} &\textbf{X vs X-Go} &\textbf{X vs X-Java} &\textbf{X vs X-Python} &\textbf{X vs X-Rust} \\
-35.0\% &11.0\% &31.3\% &-71.7\% &8.8\% \\
\textbf{X vs CPP-X} &\textbf{X vs Go-X} &\textbf{X vs Java-X} &\textbf{X vs Python-X} &\textbf{X vs Rust-X} \\
98.2\% &96.3\% &77.6\% &94.8\% &88.9\% \\
\bottomrule
\end{tabular}
\end{table}


\begin{table}[!htp]\centering
\caption{Phi-3.8}\label{tab:corrphi}
\scriptsize
\begin{tabular}{lrrrrr}\toprule
\textbf{X-CPP vs Cpp-X} &\textbf{X-Go vs Go-X} &\textbf{X-Java vs Java-X} &\textbf{X-Python vs Python-X} &\textbf{X-Rust vs Rust-X} \\
64.5\% &22.9\% &80.7\% &-9.1\% &-1.3\% \\
\textbf{X vs X-CPP} &\textbf{X vs X-Go} &\textbf{X vs X-Java} &\textbf{X vs X-Python} &\textbf{X vs X-Rust} \\
63.0\% &14.3\% &78.9\% &-10.2\% &26.9\% \\
\textbf{X vs CPP-X} &\textbf{X vs Go-X} &\textbf{X vs Java-X} &\textbf{X vs Python-X} &\textbf{X vs Rust-X} \\
99.4\% &99.5\% &98.4\% &99.9\% &95.9\% \\


\bottomrule
\end{tabular}
\end{table}
\clearpage
\newpage
Table~\ref{tab:plavg} presents the average performance with intermediate languages. Surprisingly, Rust emerges as the best intermediate language on average across all models, with natural language coming in second. For all Llama, Stable, and DeepSeek models, Rust outperforms other intermediate languages. However, for GPT models, natural language demonstrates the best performance. Compared to other popular languages such as C++, Java, and Python, Go shows better performance as an intermediate language. Conversely, Python, despite its popularity, yields the worst results. Models that are code generation based, including CodeLlama families, Stable-3b and Deepseek-1.3b, Rust is a better than natrual languages. For general purpose language model, such as GPT models and Mixtral 8x, natural language has better performance.\\

\begin{table}[!htp]\centering
\caption{Average Pass Rate of Final Generation with Different Intermediate Languages}\label{tab:plavg}
\scriptsize
\begin{tabular}{lrrrrrrrrrrrrr}\toprule
&GPT35 &GPT4 &CL7b &CL13b &CL34b &CL70b &Mixtral-7b &Mixtral-8x &Phi-3-mini &Stable-3b &Deepseek-1.3b &Average \\\midrule
Cpp &54.1\% &60.1\% &30.0\% &32.2\% &34.9\% &51.4\% &18.9\% &43.0\% &26.8\% &39.2\% &39.8\% &39.1\% \\
Go &53.4\% &55.8\% &30.8\% &35.1\% &39.3\% &52.6\% &19.4\% &40.4\% &31.9\% &40.7\% &40.9\% &40.0\% \\
Java &52.4\% &56.4\% &29.6\% &27.9\% &35.7\% &49.4\% &18.4\% &42.4\% &28.5\% &33.8\% &32.9\% &37.0\% \\
Python &50.7\% &51.2\% &25.6\% &31.1\% &36.6\% &47.3\% &18.5\% &39.0\% &27.4\% &38.6\% &39.9\% &36.9\% \\
Rust &51.2\% &62.3\% &\textbf{32.6\%} &\textbf{37.3\%} &\textbf{41.8\%} &\textbf{59.6\%} &\textbf{21.8\%} &45.3\% &34.6\% &\textbf{43.7\%} &\textbf{43.7\%} &\textbf{43.1\%} \\
NL &\textbf{57.1\%} &\textbf{65.6\%} &28.0\% &31.6\% &37.4\% &53.8\% &21.4\% &\textbf{47.1\%} &\textbf{36.8\%} &40.0\% &43.3\% &42.0\% \\
PC &51.8\% &58.3\% &28.2\% &32.2\% &35.4\% &53.7\% &19.0\% &41.6\% &34.1\% &40.0\% &34.1\% &38.9\% \\
DG &55.5\% &63.2\% &32.1\% &32.6\% &35.6\% &54.0\% &22.2\% &43.9\% &33.8\% &44.4\% &46.0\% &42.1\% \\
\bottomrule
\end{tabular}
\end{table}

\begin{table}[!htp]\centering
\caption{Average pass rate of final generation across different models }\label{tab:avg}
\scriptsize
\begin{tabular}{lrrrrrr}\toprule
&Cpp &Go &Java &Python &Rust \\\midrule
Cpp &N/A &35.6\% &46.0\% &50.2\% &24.7\% \\
Go &37.9\% &N/A &48.3\% &50.2\% &23.7\% \\
Java &37.8\% &34.1\% &N/A &51.2\% &25.1\% \\
Python &39.5\% &37.2\% &47.5\% &N/A &23.4\% \\
Rust &38.6\% &35.2\% &46.9\% &51.7\% &N/A \\
Natural language &\textbf{41.3\%} &38.3\% &\textbf{50.5\%} &53.2\% &\textbf{26.7\%} \\
Pseudo code &36.9\% &37.5\% &47.0\% &50.4\% &22.9\% \\
Direct Generation &\cellcolor[HTML]{fff2cc}41.2\% &\cellcolor[HTML]{fff2cc}\textbf{38.7\%} &\cellcolor[HTML]{fff2cc}50.0\% &\cellcolor[HTML]{fff2cc}\textbf{54.8\%} &\cellcolor[HTML]{fff2cc}25.9\% \\
\bottomrule
\end{tabular}
\end{table}


We examine the number of improvements brought by different intermediate representations. Specifically, for programming languages, we focus on cases where direct generation failed but succeeded when using an intermediate representation. The results are presented in Tables \ref{tab:improvement1} and \ref{tab:improvement2}. In Table \ref{tab:improvement1}, we ensure that the direct generation of the intermediate language is correct. In Table \ref{tab:improvement2}, we do not consider the correctness of the intermediate step. The findings indicate that, for all the programming languages studied, natural language is the most effective intermediate representation. Among the languages examined, Java and Cpp outperform Python in most cases.


\begin{table}[!htp]\centering
\caption{Average number of improvements with different programming languages.}\label{tab:improvement1}
\scriptsize
\begin{tabular}{lrrrrrr}\toprule
(1,0) -> (1,1) &Cpp &Go &Java &Python &Rust \\\midrule
Cpp &N/A &4.27 &5.00 &4.45 &7.36 \\
Go &4.82 &N/A &5.64 &5.00 &6.27 \\
Java &4.91 &6.18 &N/A &6.18 &9.82 \\
Python &0.45 &0.00 &0.00 &N/A &8.18 \\
Rust &2.36 &2.36 &3.27 &3.00 &N/A \\
\bottomrule
\end{tabular}
\end{table}

\begin{table}[!htp]\centering
\caption{Average number of improvements with different intermediate representations.}\label{tab:improvement2}
\scriptsize
\begin{tabular}{lrrrrrr}\toprule
(X,0) -> (X,1) &Cpp &Go &Java &Python &Rust \\\midrule
Cpp &N/A &11.91 &14.00 &12.09 &12.45 \\
Go &12.00 &N/A &16.18 &14.00 &12.09 \\
Java &13.09 &12.27 &N/A &12.45 &13.45 \\
Python &12.27 &13.36 &14.73 &N/A &11.82 \\
Rust &11.55 &12.73 &16.00 &14.45 &N/A \\
Natural language &\textbf{14.82} &\textbf{14.82} &\textbf{18.27} &\textbf{15.27} &\textbf{17.18} \\
Pseudo code &11.64 &12.09 &16.00 &12.91 &15.55 \\
\bottomrule
\end{tabular}
\end{table}

 
\newpage
\begin{adjustwidth}{-2.5 cm}{-2.5 cm}\centering % adjust the size
\scriptsize
\input{tables/corr}
\end{adjustwidth}
